# Supplementary material for: Turaco: Complexity-Guided Data Sampling for Training Neural Surrogates of Programs
Source: arXiv:2309.11726 source file (2023-09-21)
Supplement: Supplementary file 1 [file appendix-relational-complexity-figure.tex]

%

  %

  %

  %

  %

  %

%

%

  %

    %
  %


  %


  %
  %


%

%
%
%
%
%
%
%
%
%
%
%
%
%
%
%
%
%
%
%
%
%
%
%
%
%
%
%
%
%
%
%
%
%
%
%
%
